# Supplementary material for: Quantum Data Management in the NISQ Era: Extended Version
Source: arXiv:2409.14111 source file (2025-04-11)
Supplement: Supplementary file 1 [file appendix_TKDE.tex]

\section{Appendix}

\todo[inline]{old text, moved here from main text because we wanted it to be preserved}

\subsection{Old text from the vision section (Sec.~\ref{sec:roadmap})}

\begin{itemize}
\item{
\textcolor{darkgreen}{
%\textit{Fast decoding of error syndromes.}
\emph{Correcting errors in the quantum chip by solving a graph task.}
In the FTQC era, a large-scale error-corrected quantum computer will work in tandem with a classical computer for decoding (extracting) and correcting errors\cite{}.
A FTQC does not act on the physical qubits directly, but instead encodes the required number of qubits as logical qubits into many more physical qubits; intuitively, the resulting redundancy allows one to detect and subsequently correct errors of the logical quantum state.
The error correction procedure is performed at fixed timesteps, at which two steps are performed.
First, the classical computer tells the quantum computer to perform a specific series of $O(n)$ `check' measurements (where $n$ is the number of physical qubits), each outputting a single bit which indicates if the check found an error.
Each measurement instruction is encoded as string of $2n$ bits.
Second, decoding: the classical computer performs a minimization procedure on the joint set of measurement strings and measurement outcomes to determine the most likely error that occurred.
This error also doubles as a sequence of quantum gates which can be run on the quantum computer to correct the error.
For one of the most promising types of error correction schemes~\cite{surface-code, topological-codes}, the decoding task can be written as a Minimum Weight Perfect Matching on a weighted graph: one vertex for each measurement and the edge set and weights are constant and depend on the exact scheme used.
The most likely error corresponds to the MWPM between the vertices representing a failed check.
MWPM is generally solved in $O(n^3)$ time~\cite{} and it has been estimated an FTQC needs XXX physical qubits.
\emph{It is crucial here that the decoding, as well as the classical-quantum I/O is extremely fast, as the quantum bits in the quantum computation do not live long.}
}
\floris{The following paper seems to lay out similar challenges: \url{https://www.arxiv.org/pdf/2406.17995}.}
%\todo{note to self: mention Pauli frame?}
}
\item{
\textcolor{darkgreen}{
%\textit{Data reconciliation for secure communication.}
\emph{Secure communication requires filtering and decoding.}
Quantum bits enable unconditionally-secure communication between two network nodes~\cite{quantum-key-distribution}, by generating a classical key that the two nodes (Alice and Bob) know but is unknown to anyone else.
The most basic version of the protocol consists of: (i) Alice randomly choosing two bits and encoding these into a single qubit, (ii) sending the qubit to Bob, who (iii) randomly chooses a single bits to determine the measurement he performs on the received qubit.
The measurement outcome is a single bit.
Finally, the sifting: (iv) Alice and Bob publicly communicate one bit (Bob communicates his, and Alice communicates only the first of her two bits).
If these agree, their other bits (Bob's measurement outcome and Alice's second bit) agree and are secure with high probability.
This process is repeated until enough secure bits have been collected; in the absence of noise or someone tampering with the qubits, on average one out of every two attempts leads to a success.
For information-theoretic security~\cite{one-time pad scheme}, the key should be as long as the message $M$ the desire to send, leading to an average number of $O(2|M|)$ entries in both Alice's and Bob's local database before sifting.
However, errors on the qubits should be identified and removed; such a possible \emph{error key reconciliation} method~\cite{} is for Bob to perform a number of XYZ parity checks on the sifted key, which are sent to Alice to decode and resolve in $O(|M|^2)$ time \todo{should check}.
\tim{How is this done classically? Are classical error correction codes for classical communication stored in a database when decoded?}
}
%outputs more classical bits than only the key, part of which needs to be communicated, filtered, and mismatches should be reconciliated between parties without sacrificing security.
%Quantum cryptographic schemes for secure communication~\cite{qkd} 
}
\item{\tim{I want to add one more, let me think. Maybe `Various certification and verification procedures for checking the integrity of a quantum computation or its output', e.g. blind quantum computing (Leichtle et al.)}}
%A similar but even more complicated scheme for blind (cloud) quantum computing
\end{itemize}
